# Supplementary material for: Word-order biases in deep-agent emergent communication
Source: arXiv:1905.12330 source file (2019-06-14)
Supplement: Supplementary file 1 [file supplementary_controlLanguage.tex]

\section{Controls for long-distance and local languages}

\todo{Specify the proportion of long/local, and explain what it is precisely that you are sampling? It is a set of phrase orders, that will be constant across all possible trajectories, right? Also, give examples. Discuss Table~\ref{supp:table:examples_local} and \ref{supp:table:examples_long}}

As the long-distance language includes all utterances from the local language, it might be trivially harder to learn. To account for this, we construct $3$ control languages by randomly sampling, for each trajectory, the same number of possible utterances for the local and long-distance controls. In other words, for long-distance controls, we sample $m$ constructions,  by keeping the same proportion of local and long-distance constructions in the original long-distance language, to match the number of possible sampled utterances in the local-distance controls. Note that this number $m$ depends on the number of segments. Practically, we sample randomly $24$ possible combinations for $3$ length segments (all with local utterances for local-distance control languages and $16$ with long-distance and $8$ with local utterances for long-distance control languages) , $4$ combinations for 2-length segments and $2$ combinations for 1-length segments. 
