# Supplementary material for: Word-order biases in deep-agent emergent communication
Source: arXiv:1905.12330 source file (2019-06-14)
Supplement: Supplementary file 2 [file supplementary_earlyStopping.tex]

\subsection{The effect of early stopping in the distribution for Free order languages}
Starting iterative learning with a free word order (with markers) showed a shift from the uniform ground truth distribution to a more skewed one. We even observe this phenomenon from generation $0$. This is due to the early stopping that we impose during training. Figure \ref{fig:earlyStopping} shows the same model trained individually with early stopping (left) and to $100$ epochs (right). Both of those models have $100\%$ accuracy but the first model has a more peaked distribution with an entropy of $4.76$ compared to the second model with an entropy of $4.78$. Thus, we observe the shift from the ground truth distribution caused by the miss-match between the loss function pushing the model to fit the ground-truth distribution and the stopping criteria during evaluation that assesses the communication success. This shift becomes stronger through generations as the distribution to fit becomes less uniform.
\begin{figure}
\centering
    \includegraphics[width=\columnwidth]{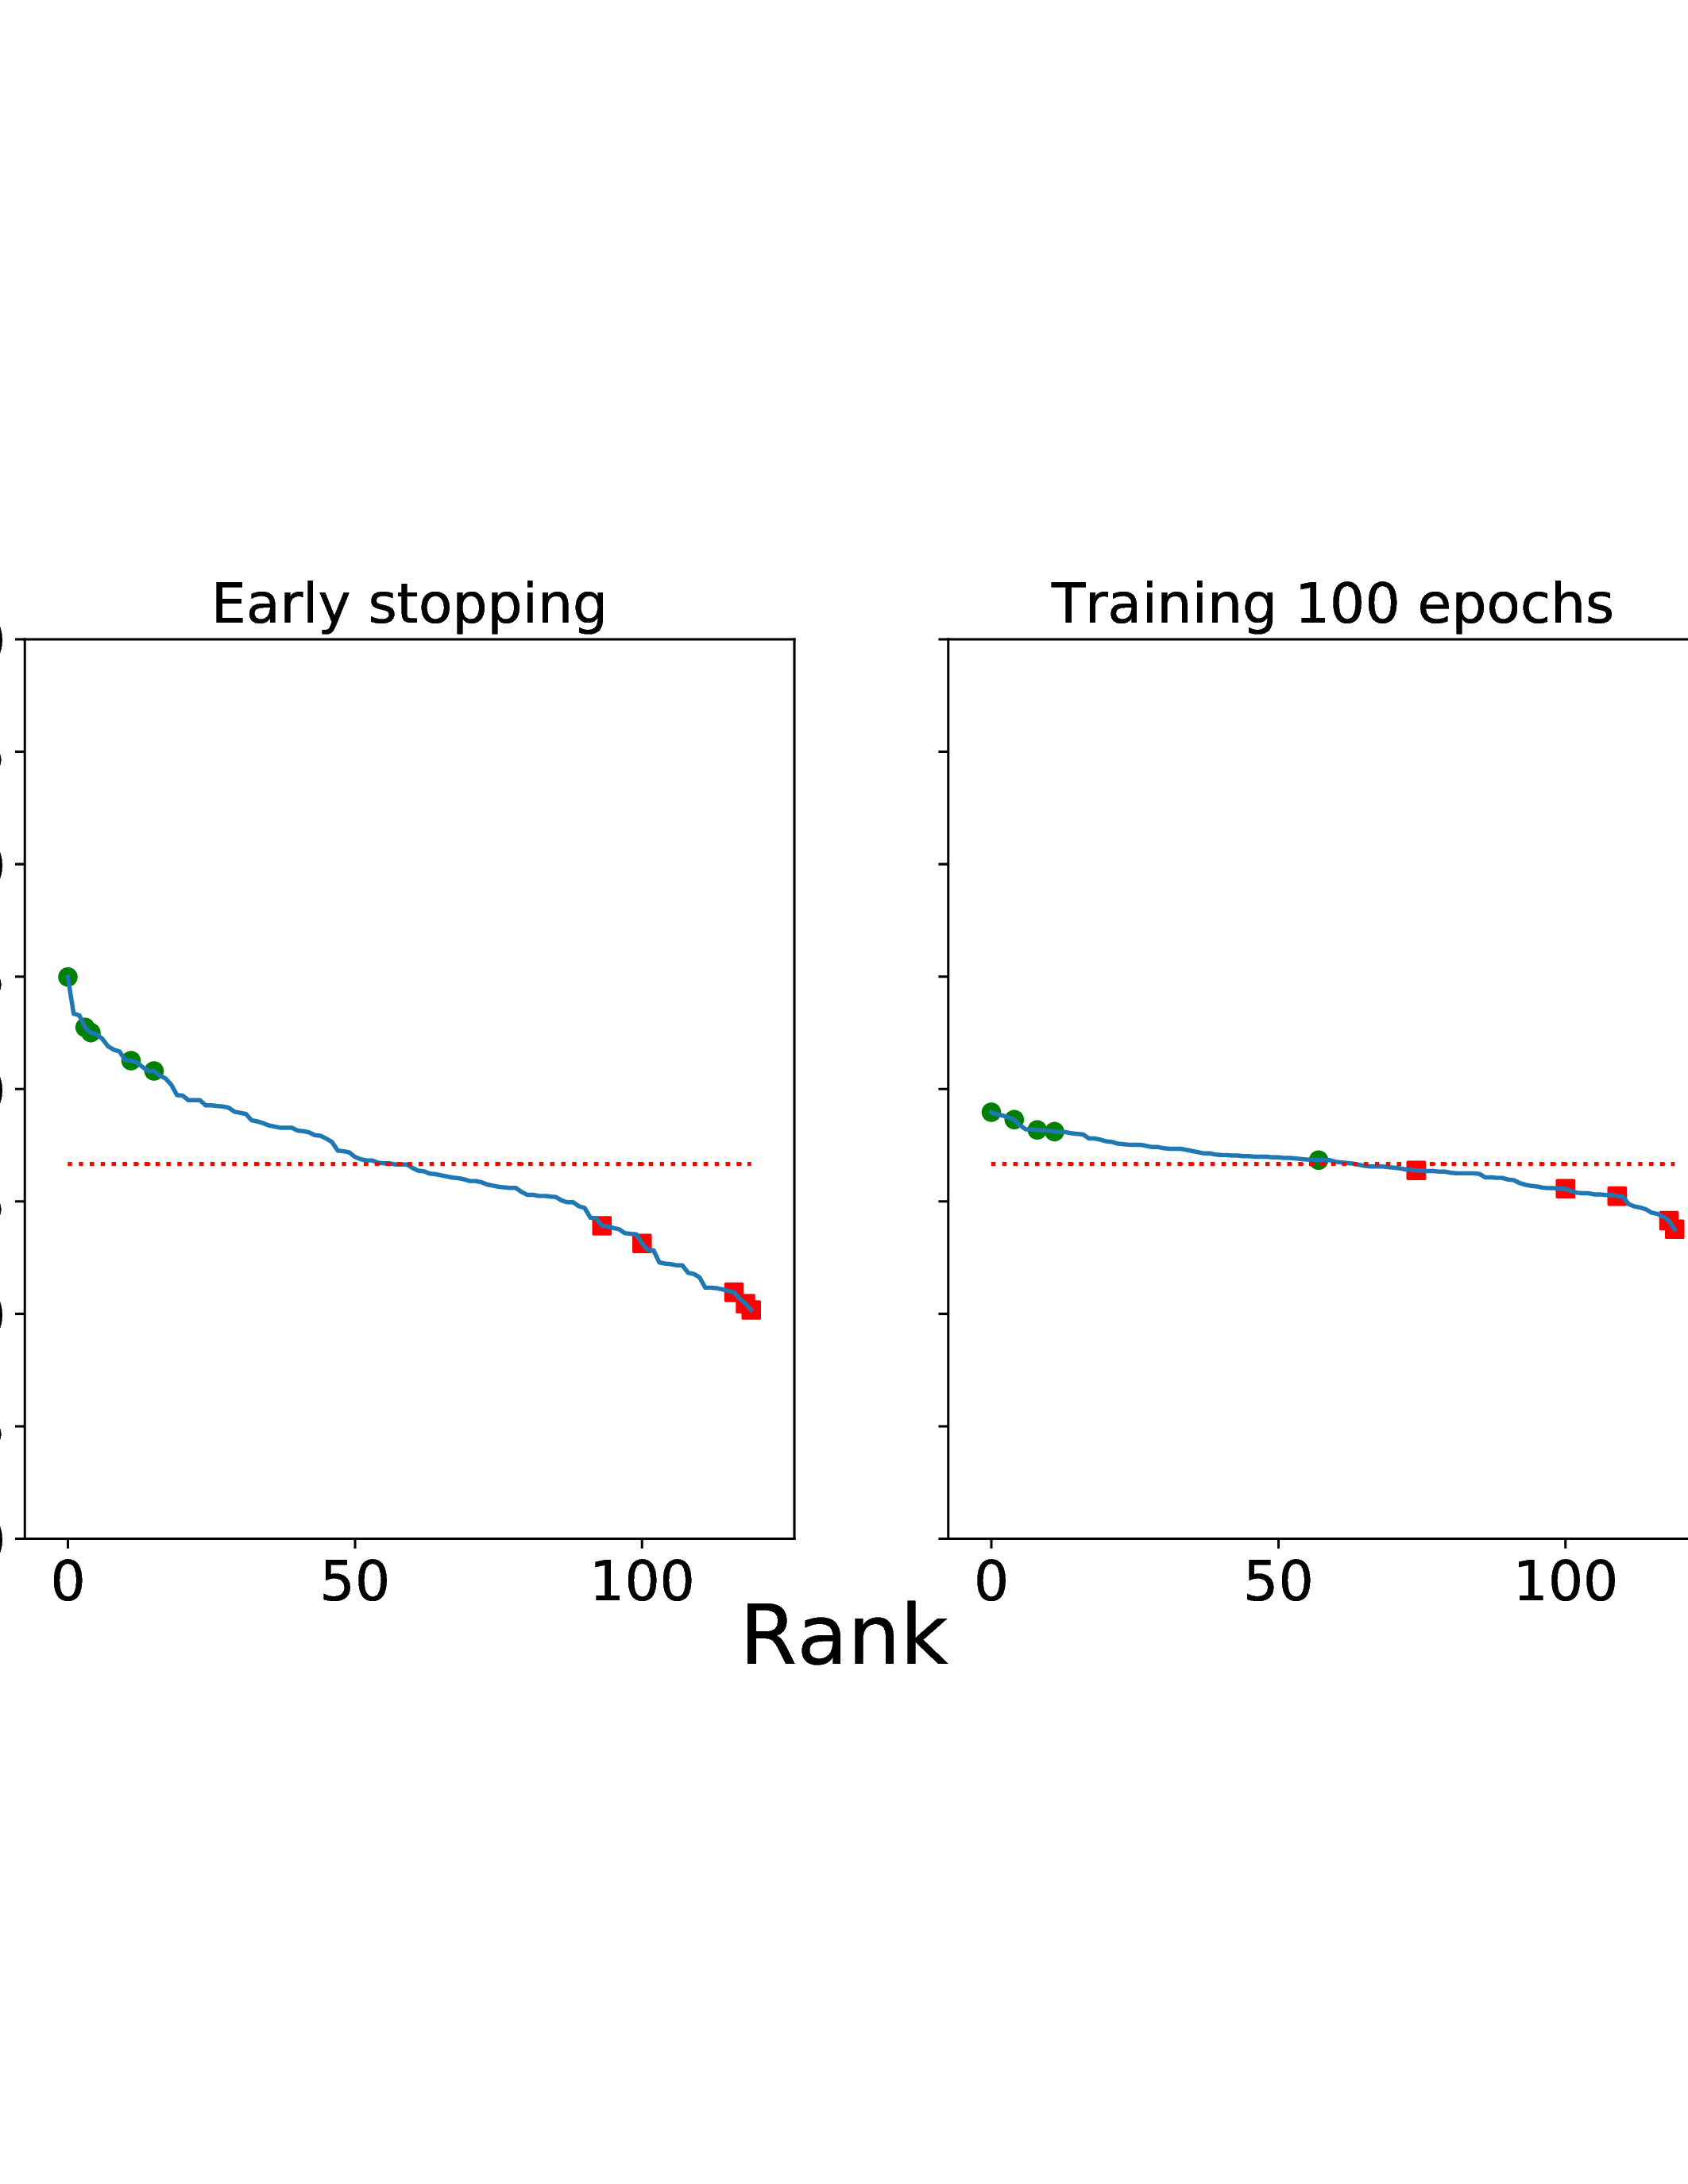}
    \caption{Distribution after convergence of models trained individually. The solid dots depict all possible order combinations that can be used to describe five-segment trajectories, sorted by their frequency (seen as a line). The dotted red line corresponds to the uniform distribution over all combinations. The most (least) frequent combination and its closest neighbours are represented by green dots (red squares).}\label{fig:earlyStopping}
\end{figure}
