# Supplementary material for: Word-order biases in deep-agent emergent communication
Source: arXiv:1905.12330 source file (2019-06-14)
Supplement: Supplementary file 3 [file supplementary_iconicityRank.tex]

\subsection{Diachronic persistence of iconic orders}

The iterative learning experiment seeded with free word-order (with markers) showed a shift from the uniform distribution of word orders.  We examine in this part some characteristics of this shift, in particular, whether backward and (forward) iconic utterances are favored through generations. We expect, that as those orders are easy for agents to acquire (fast convergence during the individual learning), they should be pushed to lower ranks through the process of evolution \footnote{Lower rank means more likely to be produced}. Practically, we launch $15$ different iteration processes starting from $3$ different seeded parents (each parent has $5$ direct children, which on their turn would have only one direct child each). Figure \ref{fig:ranks} shows the rank of production the iconic utterances. Surprisingly, we observe that the (forward) iconic order is pushed to higher ranks over generations for most seeds.  For the backward order however, we don't observe a clear pattern. The latter seems to have less variant ranks through generations, but still in contrast with our expectation, it not pushed for lower ranks. 

\begin{figure}[ht]
\centering
    \includegraphics[width=\columnwidth]{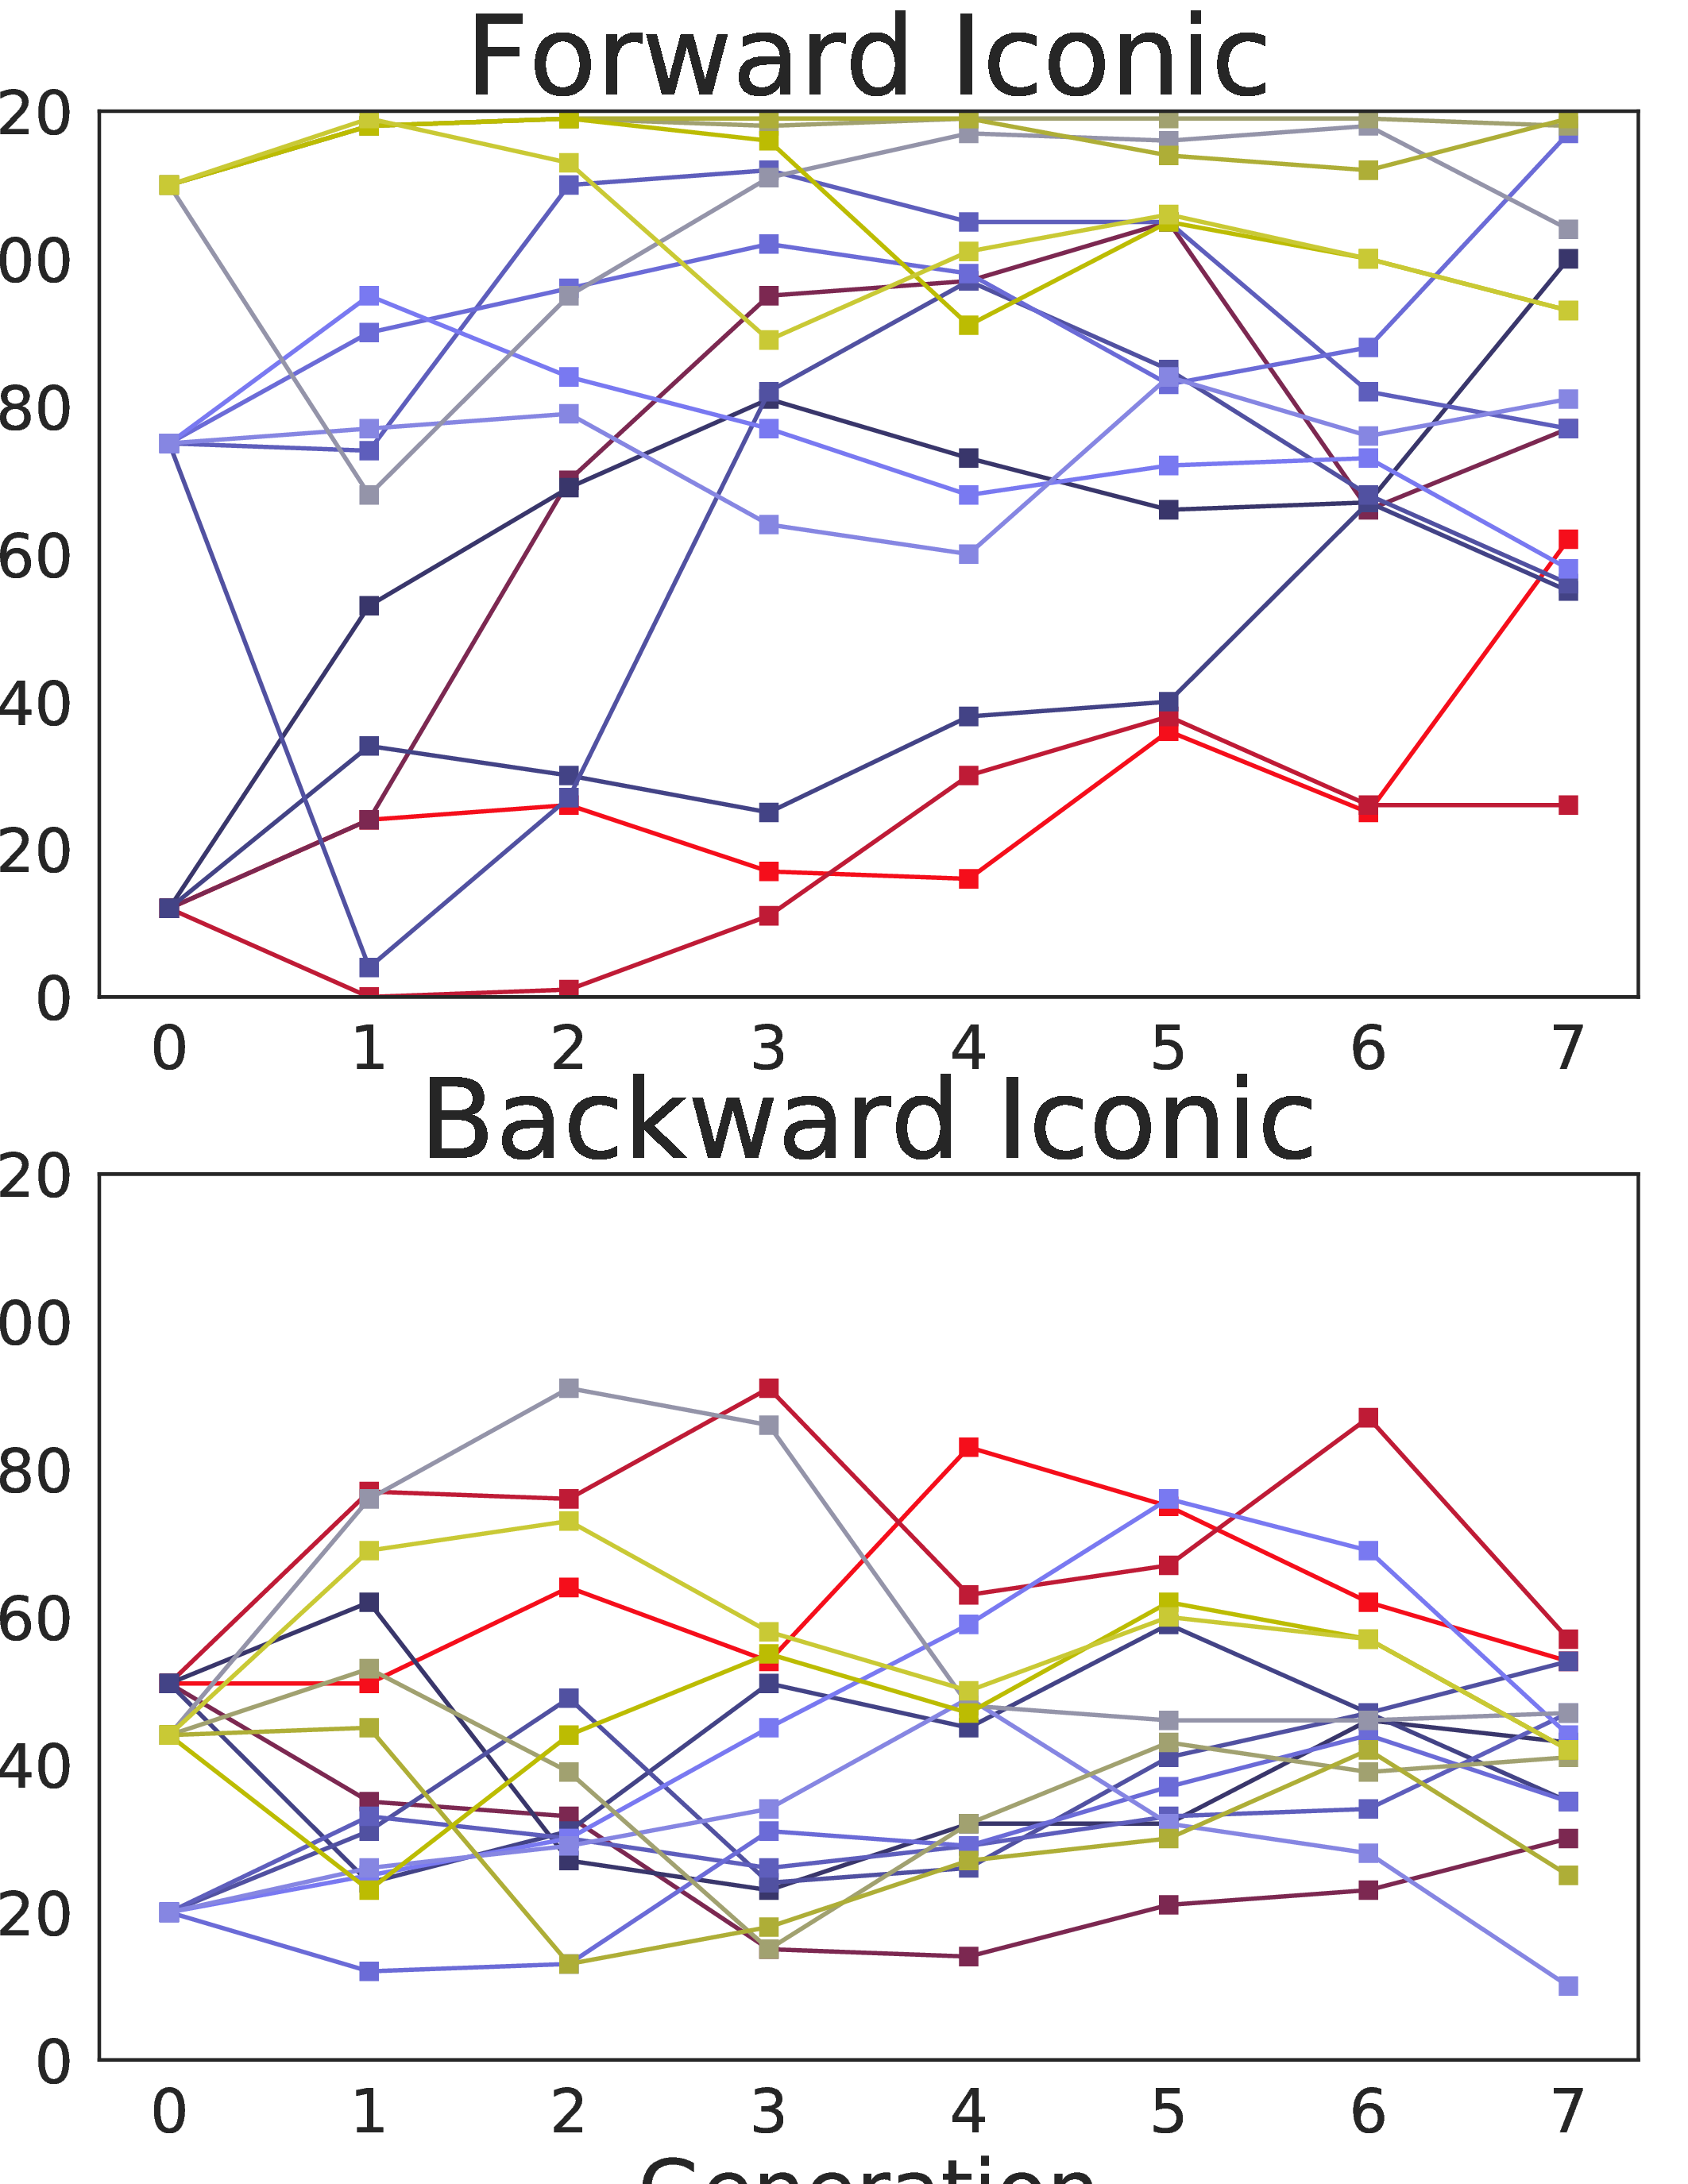}    

\caption{Rank of the production of forward (up) and backward (down) iconic orders through generations across different seeds. Each segment represents an agent and its direct successor and each color represents one iterative process from generation $0$ to $7$.}\label{fig:ranks}
\end{figure}
